# Supplementary material for: Bose-Einstein Condensation of Europium
Source: arXiv:2207.11692 source file (2022-09-23)
Supplement: Supplementary file 1 [file Bose_Einstein_condensation_of_europium_SM.pdf]

# Supplemental Material: Bose-Einstein Condensation of Europium

Yuki Miyazawa[1], Ryotaro Inoue[1], Hiroki Matsui[2], Gyohei Nomura[2], and Mikio Kozuma[1,2]
[1]*Institute of Innovative Research, Tokyo Institute of Technology, 4259 Nagatsuta, Midori, Yokohama, Kanagawa 226-8503, Japan and*
[2]*Department of Physics, Tokyo Institute of Technology, 2-12-1 O-okayama, Meguro, Tokyo 152-8550, Japan*

## I. NARROW-LINE RED-MOT

A schematic of our experimental setup (a) and the relevant energy structure (b) are shown in Fig. S1. The setup and scheme are almost identical to those of our previous work [1], which has reported the narrow-line magneto-optical trap (MOT) for Eu, except for the adoption of the stimulated Raman adiabatic passage (STIRAP [2]).

We started with a hot atomic beam of Eu in the electronic ground state $a^8\mathrm{S}_{7/2}$. The atoms were first transferred to the intermediate state $a^{10}\mathrm{D}_{11/2}$ by using STIRAP, where the Stokes laser beam at 1204 nm and the pump laser beam at 460 nm were aligned to overlap partially. The 1204-nm beam had a vertical (horizontal) beam waist of 4.8 mm (74 $\mu$m) and a power of 50 mW, whereas the 460-nm beam had a beam waist of 3.5 mm (140 $\mu$m) and a power of 10 mW. This STIRAP method allowed us to improve the transferring efficiency. The resultant atom number in our narrow-line red-MOT increases by a factor of two compared with that in our previous work [1], which utilizes the more straightforward pumping method with the aid of optical leaks from $y^8\mathrm{P}_{9/2}$ [3].

The rest of the procedure for the MOT loading is the same as reported in Ref. [1]. The atoms in $a^{10}\mathrm{D}_{11/2}$ were then optically pumped to the $a^{10}\mathrm{D}_{13/2}$ metastable state for Zeeman slowing and for capturing by a MOT (yellow-MOT [4]) using the $a^{10}\mathrm{D}_{13/2} \leftrightarrow z^{10}\mathrm{F}_{15/2}$ cooling transition at 583 nm with a natural linewidth of $\Gamma_{583}/2\pi = 8.2\,\mathrm{MHz}$. The captured atoms were successively pumped back to the ground state by driving two transitions at 609 nm and 1204 nm wavelengths. We finally loaded the atoms in $a^8\mathrm{S}_{7/2}$ to the narrow-line MOT (red-MOT) using the $a^8\mathrm{S}_{7/2} \leftrightarrow z^{10}\mathrm{P}_{9/2}$ cooling transition at 687 nm with a natural linewidth of $\Gamma_{687}/2\pi = 97\,\mathrm{kHz}$. Here, the experimental conditions for the simultaneous MOT were as follows; the detuning and total intensity of the cooling laser for the yellow-MOT were $-1.75\,\Gamma_{583}$ and $3.7\,I_{s,583}$, respectively, whereas these values for the narrow-line red-MOT were $-14\,\Gamma_{687}$ and $40\,I_{s,687}$, where $I_{s,583} = 5.4\,\mathrm{mW/cm^2}$ and $I_{s,687} = 3.9\,\mu\mathrm{W/cm^2}$ are the saturation intensities for the cooling transitions, and the axial magnetic field gradient for the MOTs was set to 3 G/cm. To plug the remaining optical leaks relevant to the red-MOT, we also illuminated the atoms by 1148-nm and 1171-nm repumpers. By the 3s-long loading with the simultaneous operation of the yellow- and the red-MOT, we obtained $8 \times 10^7$ atoms in the ground state $a^8\mathrm{S}_{7/2}$.

## II. EXPERIMENTAL SEQUENCE FOR PRODUCING BECS

Figure S2 depicts the timing sequence for the preparation of the Eu BECs. We loaded the atoms to the MOTs as described in the previous section during the first 3 s. We then plugged the atom loading by turning off the light beams relevant for the pumping, Zeeman slowing, and the yellow-MOT. In the subsequent MOT compression stage, we ramped the red-MOT parameters to load the atoms into the horizontal optical dipole trap (ODT), where the compressed MOT contains $7 \times 10^7$ atoms at a temperature of 10 $\mu$K. Afterward, we turned on the horizontal ODT beam and obtained $3.5 \times 10^6$ atoms at a temperature of 50 $\mu$K in the horizontal ODT.

In the evaporative cooling stage, the bias magnetic field $B_z = 3.00\,\mathrm{G}$ was applied to preserve the spin polarization of the atoms. The evaporative cooling was performed by gradually reducing the power of the horizontal ODT beam by 3.5 s. Next, a vertical ODT beam was introduced, and the atoms were concentrated in the crossing region within 1 s. Finally, the formation of the Eu BEC could be found by ramping down both ODT to the specific potential depth.

[1] Y. Miyazawa, R. Inoue, H. Matsui, K. Takanashi, and M. Kozuma, Phys. Rev. A **103**, 053122 (2021).
[2] K. Bergmann, H. Theuer, and B. W. Shore, Rev. Mod. Phys. **70**, 1003 (1998).
[3] Y. Miyazawa, R. Inoue, K. Nishida, T. Hosoya, and M. Kozuma, Optics Communications **392**, 171 (2017).
[4] R. Inoue, Y. Miyazawa, and M. Kozuma, Phys. Rev. A **97**, 061607 (2018).

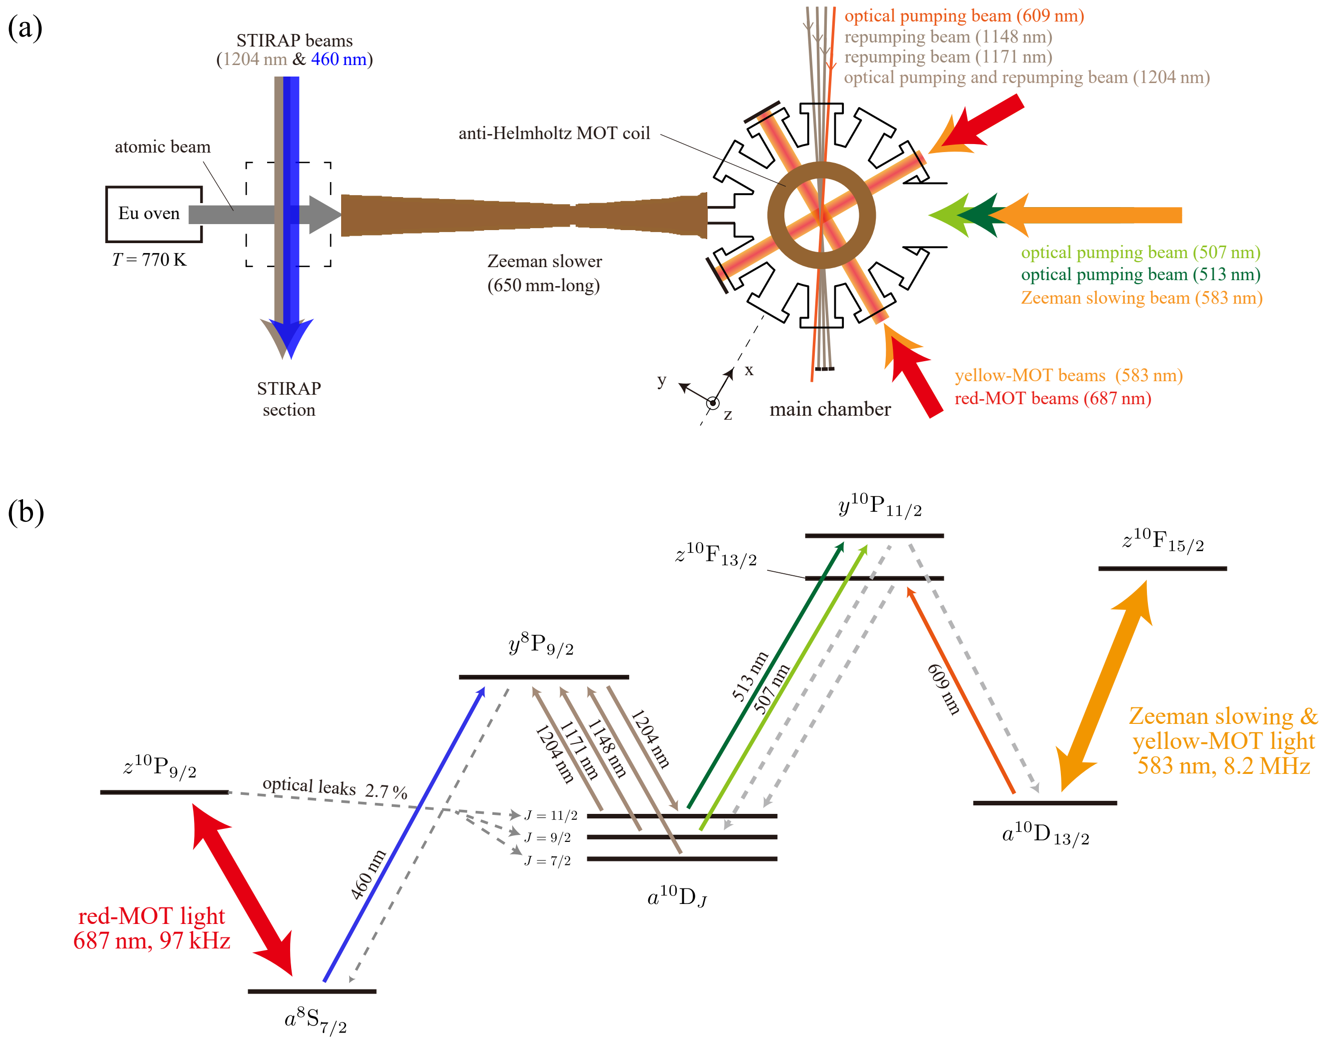


FIG. S1: (a) Experimental setup for the MOT loading stage. (b) Energy levels and transitions of Eu relevant for the MOT loading. The colored solid lines indicate laser-driven transitions, whereas gray dashed lines indicate spontaneous decay channels.

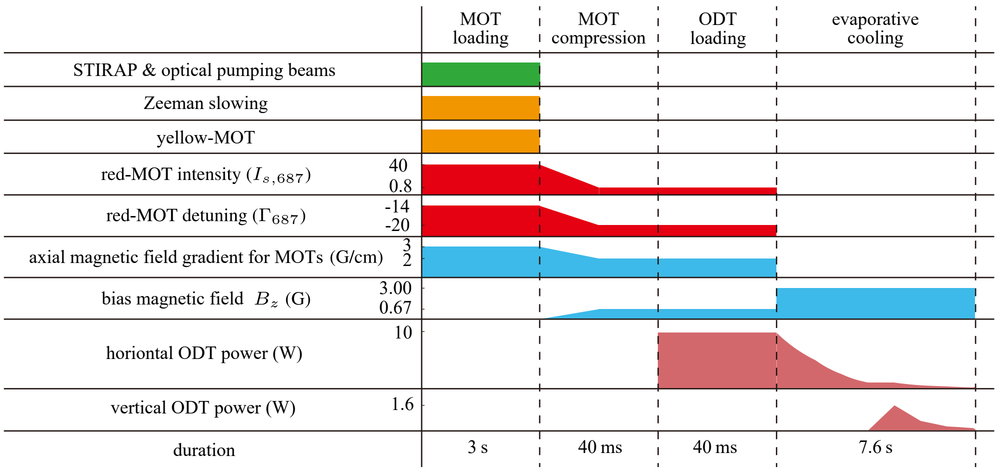


FIG. S2: Experimental control sequence for producing Eu BECs.
